# Supplementary material for: Growth of the Solid-Electrolyte Interphase: Electron Diffusion versus Solvent Diffusion
Source: arXiv:2209.10854 ancillary file (2022-09-22)
Supplement: Supplementary file 1 [file SupplementaryInformation.pdf]

# Supplementary Information to "Growth of the Solid-Electrolyte Interphase: Electron Diffusion versus Solvent Diffusion"

Lukas Köbbing<sup>a,b</sup>, Arnulf Latz<sup>a,b,c</sup>, Birger Horstmann<sup>a,b,c,\*</sup>

<sup>a</sup>*Institute of Engineering Thermodynamics, German Aerospace Center (DLR), Wilhelm-Runge-Straße 10, 89081 Ulm, Germany*

<sup>b</sup>*Helmholtz Institute Ulm (HIU), Helmholtzstraße 11, 89081 Ulm, Germany*

<sup>c</sup>*Institute of Electrochemistry, Ulm University, Albert-Einstein-Allee 47, 89081 Ulm, Germany*

## 1. Capacity loss at SOC=0% for Keil et al. [1]

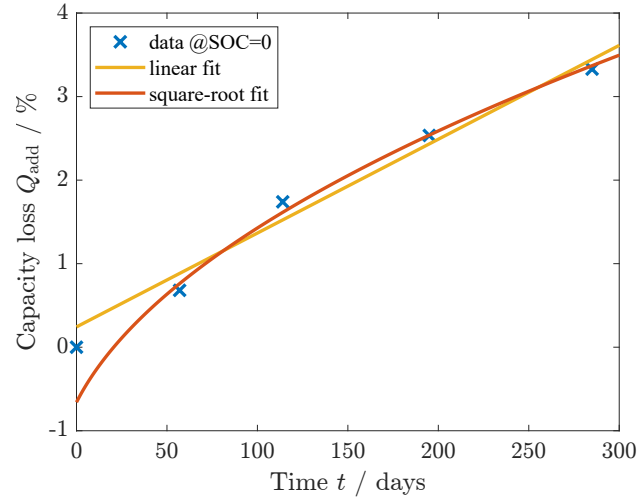

Figure SI-1: Capacity loss at SOC = 0% measured in Ref. [1]. We assume the initial capacity loss  $Q_{\text{SEI},0} = 1\%$ .

\*birger.horstmann@dlr.de

## 2. Capacity loss at SOC=0% for Naumann et al. [2]

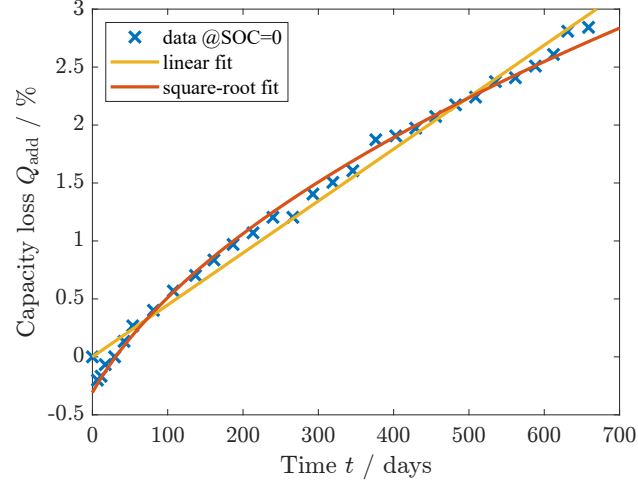

Figure SI-2: Capacity loss at SOC = 0% measured in Ref. [2]. We assume the initial capacity loss  $Q_{\text{SEI},0} = 1\%$ .

### 3. Electron diffusion describing the capacity loss for Naumann et al. [2]

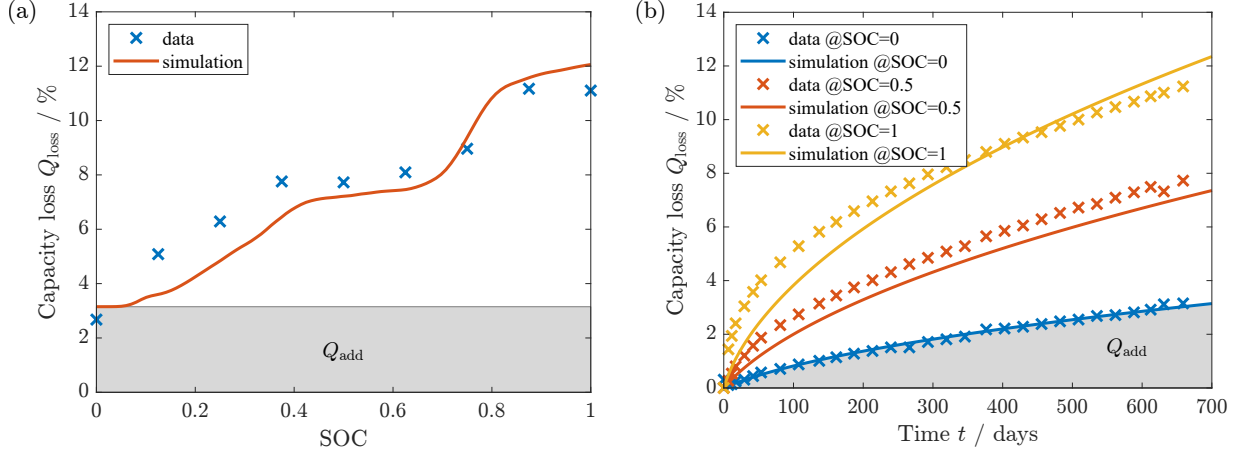

Figure SI-3: Capacity loss simulated with electron diffusion fitted to the SOC depending data measured in Ref. [2]. (a) Capacity loss depending on the SOC. Agreement between simulation and data is reasonable, although the exact curve for the anode open circuit voltage is not known. (b) Capacity loss depending on time. The agreement is excellent at low SOC, while at medium SOC, the general time behavior is reproduced, but the simulated values overall are too low. At high SOC, the simulation shows a large deviation from the data points.

#### 4. Solvent diffusion describing the capacity loss for Naumann et al. [2]

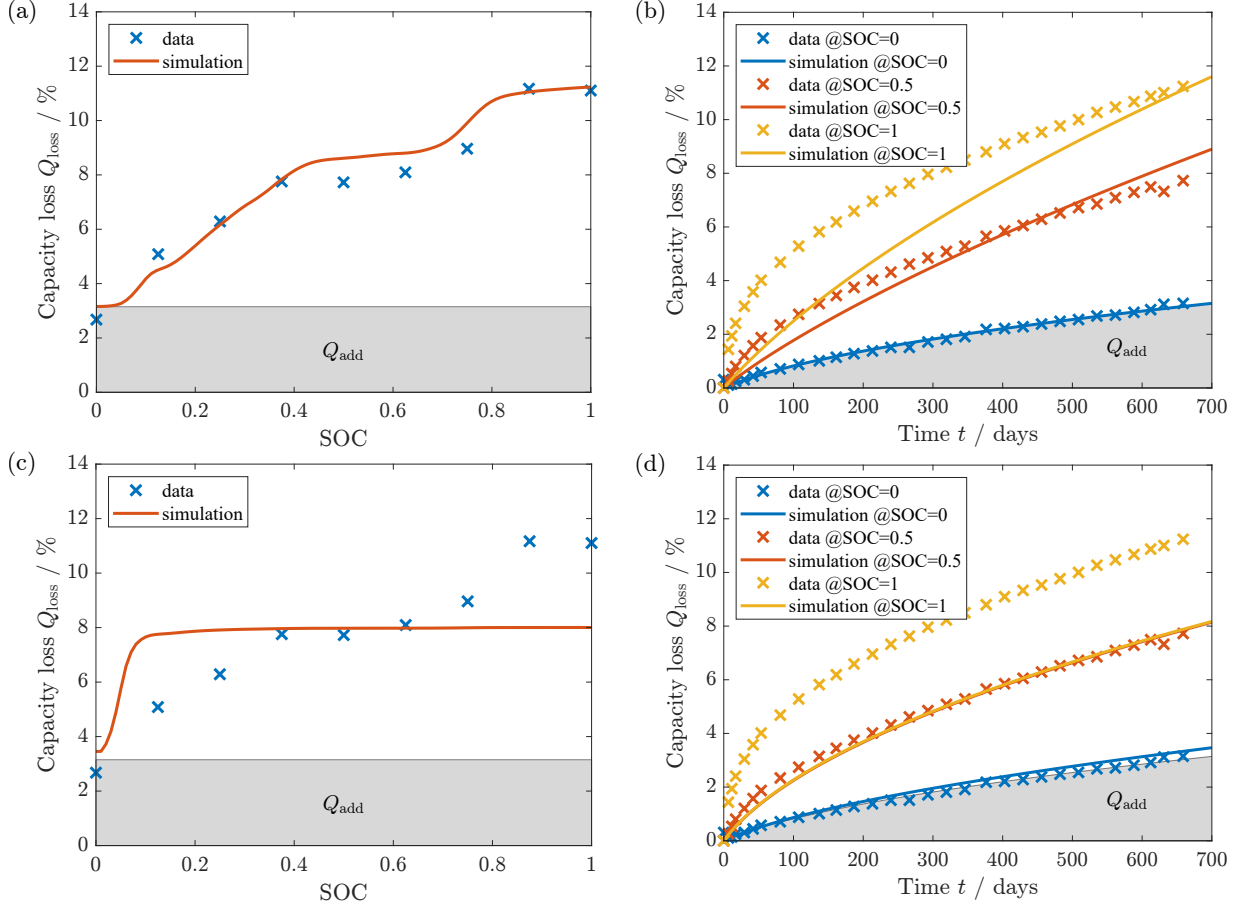

Figure SI-4: Capacity loss simulated with solvent diffusion in comparison to the data measured in Ref. [2]. (a) and (b) Fit of the solvent diffusion model to the SOC dependence of capacity loss (a) Capacity loss depending on the SOC. The agreement between simulation and data points is reasonable. (b) Capacity loss depending on time. Simulation and experiment do not match at medium and high SOC. (c) and (d) Fit of the solvent diffusion model to the time dependence of capacity loss at SOC = 50% (c) Capacity loss depending on the SOC. The observed dependence is not captured at all. (d) Capacity loss depending on time. Good agreement is achieved at SOC = 50%, but the simulation does not reproduce the behavior at SOC = 100%.

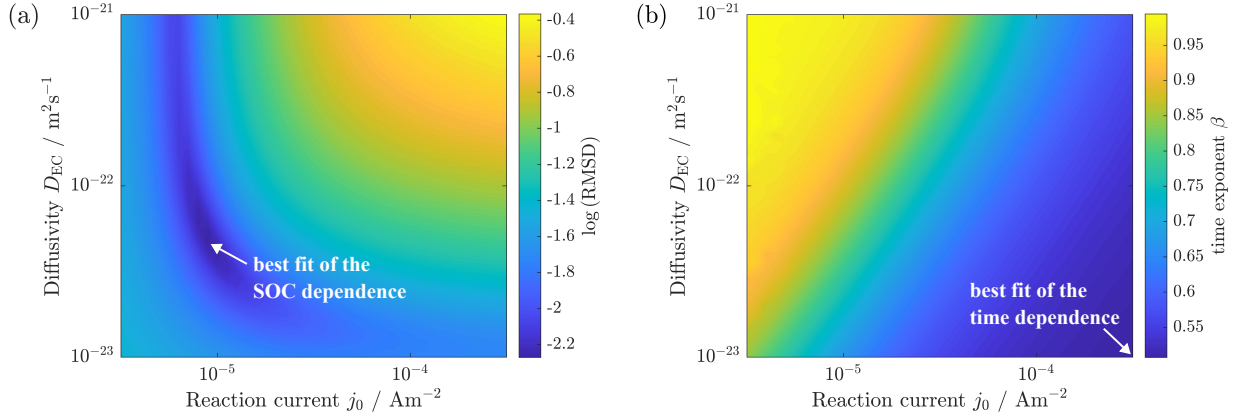

Figure SI-5: Parameter study for the capacity loss simulated with solvent diffusion with a variation of the reaction current  $j_0$  and the diffusion coefficient  $D_{EC}$ . (a) Logarithm of the root mean square deviation of the simulated capacity loss depending on the SOC from the experiment [2]. The smallest deviation is depicted in dark blue and reached for small reaction current  $j_0$  and medium diffusivity  $D_{EC}$ . The best fit of the SOC dependence with the parameters used in Fig. SI-4(a) is highlighted. (b) Fitted time exponent  $\beta$  to the simulation. The experiment can be approximately described with  $t^{0.5}$  depicted in dark blue. Either large values of  $j_0$  or small values of  $D_{EC}$  are needed to achieve a good agreement with  $t^{0.5}$ . The best fit of the time dependence with the parameters used in Fig. SI-4(d) is highlighted.

## References

- [1] P. Keil, S. F. Schuster, J. Wilhelm, J. Travi, A. Hauser, R. C. Karl, A. Jossen, [Calendar Aging of Lithium-Ion Batteries](#), Journal of The Electrochemical Society 163 (9) (2016) A1872–A1880. doi:10.1149/2.0411609jes. URL <https://iopscience.iop.org/article/10.1149/2.0411609jes>
- [2] M. Naumann, M. Schimpe, P. Keil, H. C. Hesse, A. Jossen, [Analysis and modeling of calendar aging of a commercial LiFePO<sub>4</sub>/graphite cell](#), Journal of Energy Storage 17 (2018) 153–169. doi:10.1016/j.est.2018.01.019. URL <https://doi.org/10.1016/j.est.2018.01.019https://linkinghub.elsevier.com/retrieve/pii/S2352152X18300665>
